# Supplementary material for: ARShopping: In-Store Shopping Decision Support Through Augmented Reality and Immersive Visualization
Source: arXiv:2207.07643 source file (2022-07-15)
Supplement: Supplementary file 1 [file 10-appendix.tex]

\section*{Appendix}
\begin{figure}[h]
\includegraphics[width=8cm]{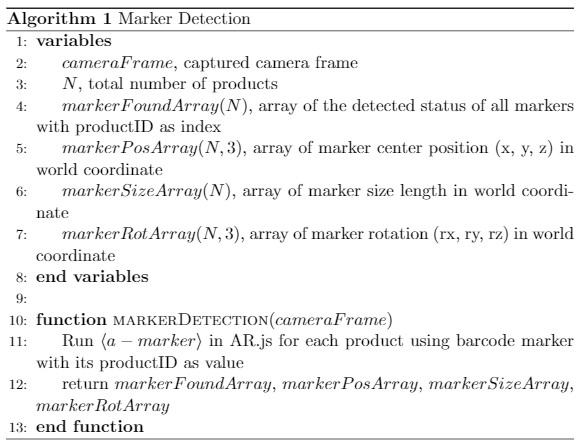}
\centering
\end{figure}

\begin{figure}[h]
\includegraphics[width=8cm]{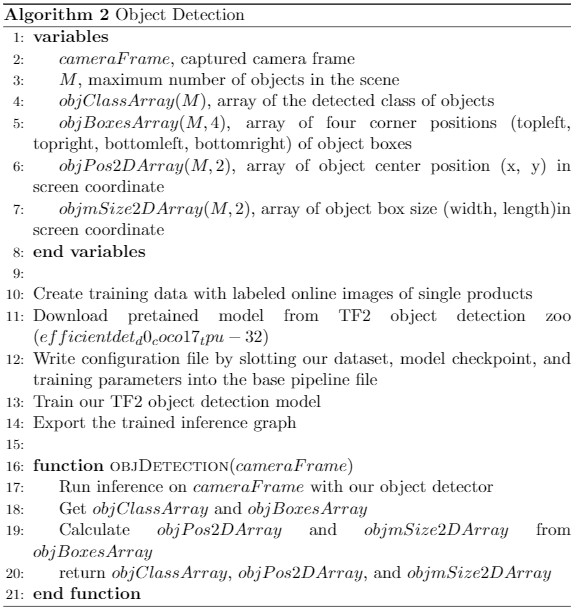}
\centering
\end{figure}

\begin{figure}[h]
\includegraphics[width=8cm]{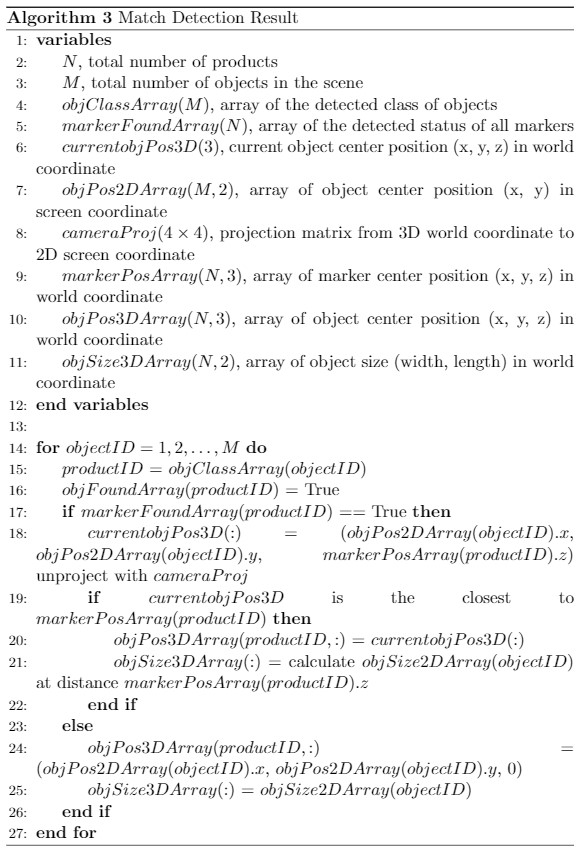}
\centering
\end{figure}

\begin{figure}[h]
\includegraphics[width=8cm]{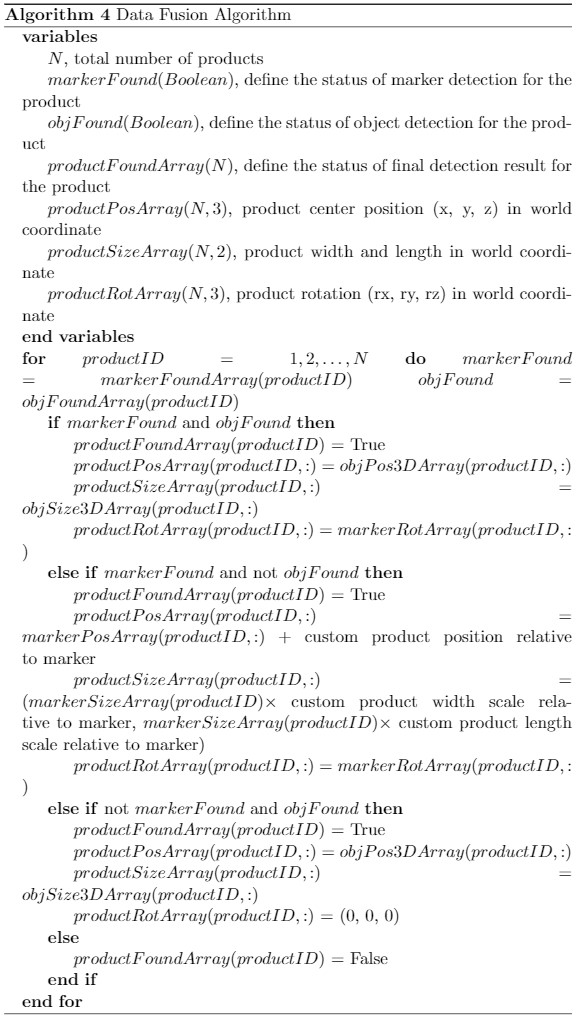}
\centering
\end{figure}
